# Supplementary material for: Motion Planning on Visual Manifolds
Source: arXiv:2210.04047 source file (2024-02-19)
Supplement: Supplementary file 1 [file figures_appendix.pdf]

# Topology (Veeramani) Chapter 1

# Open Intervals are Open Sets

$\mathbb{R}$ : Real line

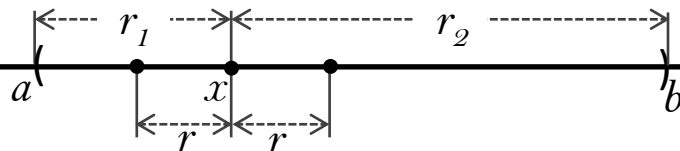

# Basis of a Topology

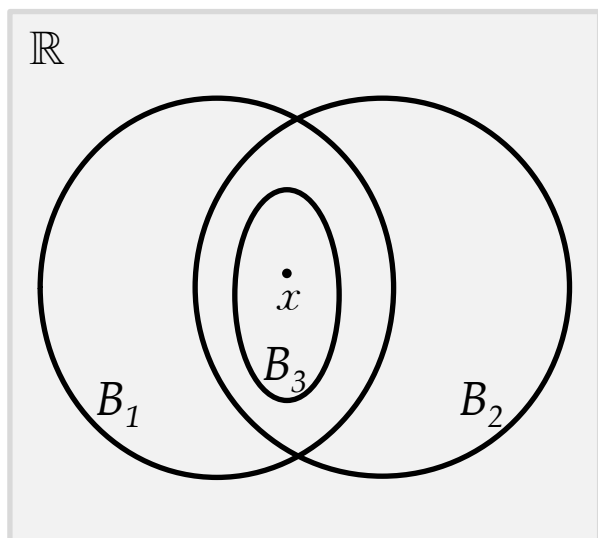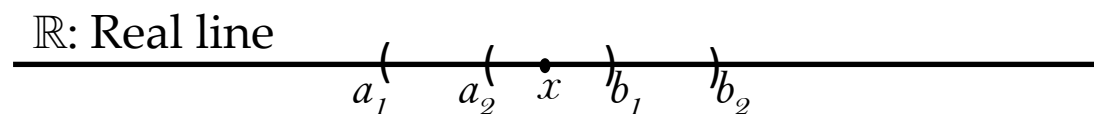

# Topology Generated by a Basis

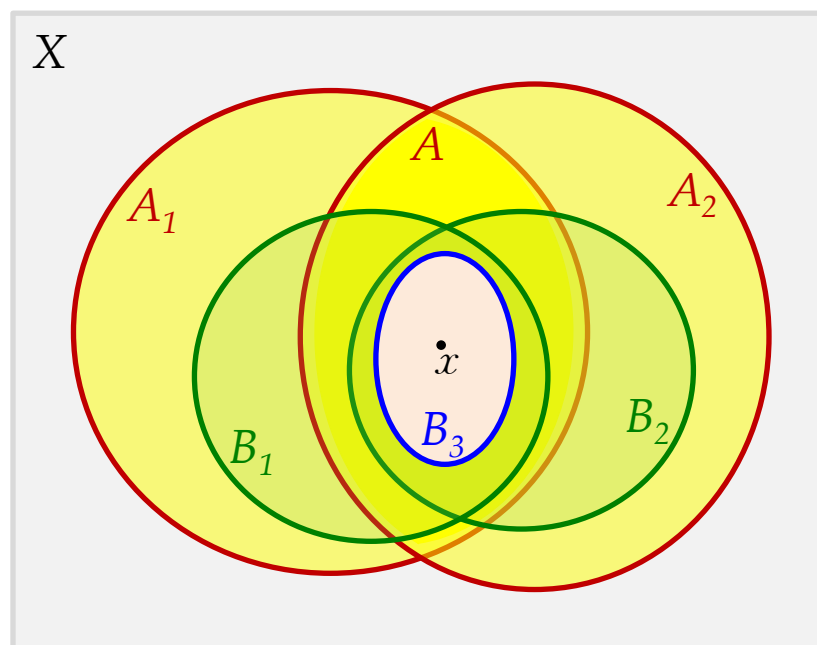

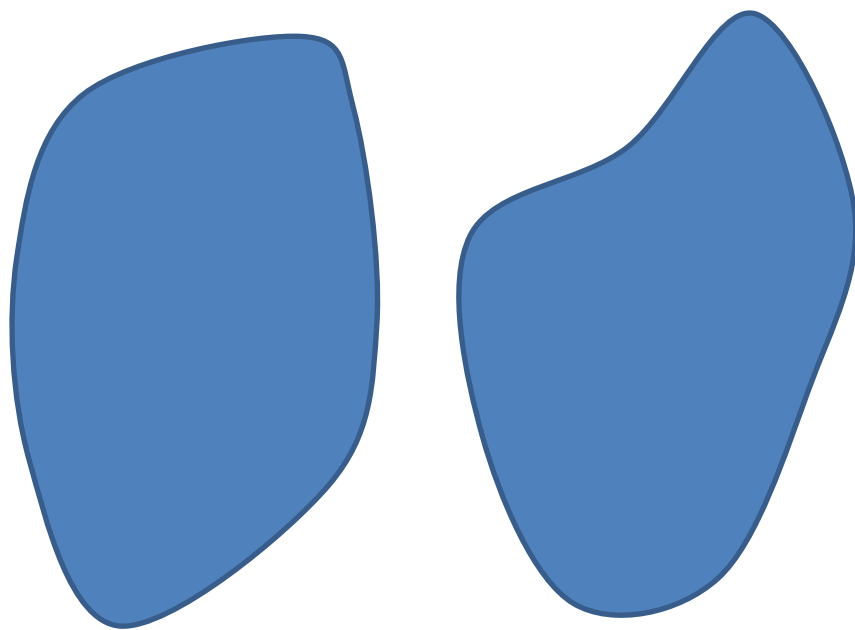

If  $B_1 = (a_1, b_1)$ ,  $B_2 = (a_2, b_2)$ , then  $\forall x \in (a_1, b_1) \cap (a_2, b_2)$ ,  
by taking  $B_3 = (a_2, b_1)$ , we have  $x \in B_3 \subseteq B_1 \cap B_2$ .
